# Supplementary material for: QuickSel: Quick Selectivity Learning with Mixture Models
Source: arXiv:1812.10568 source file (2020-04-10)
Supplement: Supplementary file 1 [file additional_discussion.tex]

\ignore{
\section{Join Selectivity \& Other Types}
\label{sec:prelim:join}

Query-driven selectivity estimation can be generalized in two orthogonal directions: (1) estimating the selectivity of a query including joins and (2) supporting more data types.

\ph{Selectivity for Join\texttt{+}Selection}
\cref{prob:sec} concerns the selectivity only for a single relation. However, the selectivity of a joined relation can also be computed by combining the selectivity estimates on a single relation and the selectivity of join conditions, under the assumption that the join conditions are independent of the selection predicates placed on individual tables~\cite{oracle_cbo}. For example, suppose that two predicates $P_1$ and $P_2$ are respectively placed on two relations $T_1$ and $T_2$, which are inner-joined on $T_1.C = T_2.C$.
Then, one heuristic rule for the inner-join selectivity is $s_{join} = 1 / \max(|\text{distinct}(T1.C)|, |\text{distinct}(T2.C)|)$~\cite{spark_cbo}. 
Let $s_1$ and $s_2$ be the selectivities of $P_1$ and $P_2$, respectively. Then, the number of the tuples of the joined relation can be computed as $|T_1| \cdot |T_2| \cdot s_{join} \cdot s_1 \cdot s_2$. This approach can also be applied to the other join selectivity rules~\cite{postgres_cbo,haas1996selectivity,van1993multiple}.

\ph{Other Data Types}
\cref{prob:sec} can be extended to support the relations containing discrete attribute values (e.g., integer, char) and the equality constraints on them, as follows. Without loss of generality, suppose that the domain of $C_i$ is $\{ 1, 2, \ldots, b_i \}$. Then, the constraint ``$C_i = k$'' is converted to the range constraint $k < C_i < k+1$; the domain of $C_i$ is converted to $(1, b_i + 1)$. Mathematically, this is equivalent to replacing a probability mass function with a probability density function consisting of \emph{dirac delta functions}.\footnote{A dirac delta function $\delta(x)$ outputs $\infty$ if $x = 0$ and outputs 0 otherwise while satisfying $\int \delta(x)\, dx = 1$.} Then, the summation of the original probability mass function can also be converted to the integration of the probability density function.
Moreover, the string data types (e.g., char, varchar) and the equality constraints on them can also be supported by internally maintaining a mapping from a string value to an integer and applying the technique described above for the integer data type.
}

\ignore{
\section{Warm Start}
\label{sec:training:warm}

One shortcoming of \method is that its accuracy can be low when the number of \emph{relevant} observed queries is small. This occurs in two cases: first, a relation was recently created, and not enough observed queries have been collected for the relation; second, the new workload significantly differs from the past workloads, rendering most past observed queries uninformative.

We can address this cold-start problem by incorporating existing static techniques (e.g., histograms~\cite{spark_cbo,sqlserver_cbo,ibm_cbo,oracle_online,gunopulos2005selectivity,ilyas2004cords,gunopulos2000approximating} or Most Common Values~\cite{postgres_cbo}) into query-driven selectivity estimation, as follows.

\ph{Histograms} The buckets constructed by any histogram construction algorithms, including equi-width, equi-depth, etc., can be expressed as observed queries in a straightforward way. For example, if 10\% tuples are included within the range (0,10), the range is a special case of a hyperrectangle (for a predicate) and the frequency is the selectivity. These information can then simply be incorporated in the observed query list of the query-driven selectivity estimation problem (\cref{prob:sec}).

\ph{Most Common Values} Most common values (MCVs) capture the frequency of high-frequency attribute values. For example, if a string value \texttt{'AAA'} appears in 2\% of the tuples (in a certain attribute), a pair (\texttt{'AAA'}, 0.02) is stored and used for selectivity estimation. Note that this is also a special case of an observed query. We already described how to handle the equality conditions in \cref{sec:prelim:join}.
}

\section{Relationship to Max Entropy}
\label{sec:disc:entropy}

The max-entropy query-driven histograms optimize their parameters (i.e., bucket frequencies) by searching for the parameter values that maximize the entropy of the distribution $f(x)$. We show that this approach is approximately equivalent to \method's optimization objective, i.e., minimizing MSE of $f(x)$ from a uniform distribution. The entropy of the probability density function is defined as $\minus \int f(x) \, \log( f(x) ) \, dx$. Thus, maximizing the entropy is equivalent to minimizing $\int f(x) \, \log( f(x) ) \, dx$, which is related to minimizing MSE as follows:
\begin{align*}
  \argmin \int f(x)\,  \log( f(x) ) \; dx 
  &\approx \argmin \int f(x)\, (f(x) - 1) \; dx \\
  &= \argmin \int (f(x))^2 \; dx
\end{align*}
since $\int f(x) \, dx = 1$ by definition. We used the first-order Taylor expansion to approximate $\log(x)$ with $x - 1$. Note that, when the constraint $\int f(x)\, dx = 1$ is considered, $f(x) = 1/|R_0|$ is the common solution to both the entropy maximization and minimizing MSE.
