# Supplementary material for: QuickSel: Quick Selectivity Learning with Mixture Models
Source: arXiv:1812.10568 source file (2020-04-10)
Supplement: Supplementary file 2 [file additional_exp.tex]

\input{fig_tab/fig_exp_param}

\section{Additional Experiments: Impact of Data Correlation, Workload, and Parameter Count Control}
\label{sec:exp:param}
\barzan{prev subsection already talked about param count.
why r u flip flopping?}

We further studied how \method's accuracy is affected by data distribution, query workload distribution, and the number of its model parameters. 
\tofix{To control the number of model parameters, we manually controlled \method rather than using its default option (i.e., \# of model params = 4 $\times$ \# of observed queries).}

\ph{\tofix{Sensitivity to Data Correlation}}
To study how \method's accuracy changes based on different data \tofix{correlations}, we used \synthetic with different correlations. 
\tofix{In each case, \method trained its model using 100 observed queries; the error was measured using 100 different queries.}
\barzan{u say to study diff dists we used this one dist w diff params!!!}
As shown in \cref{fig:exp:param:a}, 
    the errors were almost identical \tofix{for all cases with different correlations.}
    % except when
    % the correlation was considerably higher 
    % (i.e., $\geq$0.9). 
    
    % This is because, when the correlation is high, 
    %     only a small number of assertions are actually useful \tofix{(i.e., the probability distribution is almost zero for most areas)}, 
    %     \yongjoo{Make a connection here.}
    %     which leads to slightly lower accuracy. 
    %     Nevertheless, \method still produced highly accurate estimates even under high correlations (i.e., less than 0.5\% error).

\ph{Workload Shifts}
We also studied  \method's accuracy 
under situations where the 
query workload shifts over time. 
Here, we generated the  \synthetic dataset
with
% data points using a bivariate normal with mean (0.5, 0.5) and 
correlation 0.5.
We generated  queries with different predicates,
    with each predicate being a different rectangle in the 2-dimensional 
    space.\footnote{\tofix{The purpose of this synthetic dataset is to 
        simulate a workload shift, we study high-dimensional data and queries in \cref{fig:exp:param:d}.}}
We simulated three scenarios of workload shifts
    by modifying these rectangular predicates. 
First, we created a \emph{random-shift} workload by choosing random rectangles in the space. We also created a \emph{sliding-shift} workload by gradually moving the rectangles from the left-tail of the normal
        distribution towards the right-tail.
Third, we created a \emph{no-shift} workload by using the same rectangle for all queries.

 %To catest \method's accuracy, this experiment used a slightly different approach.
In each scenario, we first trained \method on the first 10 observed queries (i.e., sequence numbers: 1--10) and   measured the accuracy on the next 10 observed queries (i.e., sequence numbers: 11--20). 
Then, we trained \method on the first 20 observed queries (i.e., sequence numbers: 1--20) and measured the accuracy using the next 10 observed queries (i.e., their sequence numbers: 21--30). We kept increasing the number of observed queries until we reached 
    1,000 observed queries for training.
The results are plotted in \cref{fig:exp:param:b}. 

\barzan{this para should change} \yongjoo{Changed}
\tofix{As expected, the errors were highest for random shift workload. However, the error gradually decreased as \method observed more queries; when 100 queries were observed, the relative error was only 1.2\% for the random shift workload. The errors were lower in general for other workloads.}

% \tofix{Initially, the errors were lower for the shifting workload, which was only because the queries around the bottom-left corner were associated with low selectivities (thus, lower absolute errors). However, the errors for the static workload decreased quickly. In contrast, the errors for the shifting workloads elevated slightly. Nevertheless, the errors were low in general (i.e., less than 0.5\%). The primary reason \method yielded low errors, even for the \emph{new} areas, was that \method exploited the global property of every probability distribution. That is, the probability distribution function must sum (or integrate) to one, which is reflected in \method's optimization constraint; thus, learning the probability distribution of one area also refines the probability distribution estimates for the other areas, even though the other areas are never queried.}

\ph{Model Parameter Count}
Third, we studied the relationship between the number of model parameters and \method's accuracy, \tofix{with a fixed number of observed queries: 100}. 
% Recall that the 
% number of \method's parameters can be         controlled by 
%     choosing the number of centers in its $k$-means clustering (\cref{sec:model:sub}).
% Here, we used 100 queries for training; 
The dataset 
was \synthetic with correlation 0.5.
\cref{fig:exp:param:c} shows the results. 
As expected, the errors were relatively higher when the number of model parameters was extremely small (i.e., 10). 
However, as soon as the number of model parameters reached 50 the error
    was drastically reduced.

\ph{Column Set Size}
\tofix{
Lastly, we studied the relationship between the \emph{column set size} and the error of \method; \method approximates the join distribution of the column set.
For this experiment, we generated the datasets from multivariate normal distributions; for each dataset, we generated queries with the same average selectivities and used them for both training and tests.

\cref{fig:exp:param:c} shows the result. For comparison, we also report the error of AutoSample, which is not sensitive to the data dimension by nature. In the figure, \method was more accurate than AutoSample when the column set size was less than 8 while the error of \method was larger than AutoSample for bigger column sets.

Note that this property of \method does not reduce its practical usefulness
since the selectivity of a big column set can be estimated by the selectivities of smaller columns sets that partitions the big column set~\cite{oracle_cbo,postgres_cbo}.
}
